# Supplementary material for: Knowledge Distillation with Multi-granularity Mixture of Priors for Image Super-Resolution
Source: arXiv:2404.02573 source file (2024-04-03)
Supplement: Supplementary file 2 [file rand-sampler.tex]

\begin{table}[]
\caption{Ablation for the frequency of random propagation of the Block Prior Mixer. The RCAN student model of c64b5g10 is distilled by the teacher model of c64b6g10.}
\label{tab:rand-sampler}
\centering
\begin{tabular}{@{}ccccccccc@{}}
\toprule
\multirow{2}{*}{\#propagation per sample} & \multicolumn{2}{c}{Set5} & \multicolumn{2}{c}{Set14} & \multicolumn{2}{c}{BSD100} & \multicolumn{2}{c}{Urban100} \\ \cmidrule(l){2-9} 
                                       & PSNR       & SSIM        & PSNR        & SSIM        & PSNR        & SSIM         & PSNR         & SSIM          \\ \midrule
1                                      & 31.99      & 0.8919      & 28.43       & 0.7777      & 27.46       & 0.732        & 25.69        & 0.7728        \\
2                                      & 31.87      & 0.8884      & 28.38       & 0.7632      & 27.42       & 0.7311       & 25.62        & 0.7699        \\
4                                      & 31.86      & 0.8867      & 28.37       & 0.7619      & 27.41       & 0.7306       & 25.57        & 0.7697        \\ \bottomrule
\end{tabular}
\end{table}
